# Supplementary material for: Implicit Interpretation of Importance Weight Aware Updates
Source: arXiv:2307.11955 source file (2023-07-22)
Supplement: Supplementary file 1 [file appendix.tex]

\section{Appendix}
\label{sec:appendix}
